# Supplementary material for: Handling missing data in Burundian sovereign bond market
Source: arXiv:2309.17379 source file (2023-09-29)
Supplement: Supplementary file 1 [file appendix.tex]

\section*{Appendix}
Two other risks to which a bond is exposed are liquidity risk and interest rate risk.

\textbf{UEMOA}: West African Economic and Monetary Union

\textbf{CIPRES}: Inter-African Conference on Social Security

In six years, the share of debt in the form of treasury securities in domestic public debt has almost
doubled: from 32\% in 2014 to 61\% in 2020. Source: \url{http://www.brb.bi/fr/content/finances-publiques}. Accessed on 28/12/2021.

Institutional investors include all non-bank financial intermediaries, i.e. Undertakings for Collective
Investment in Transferable Securities (UCITS, in acronym; there are none at present but they are provided for
in the Capital Market Act), insurance companies and pension funds.
